# Supplementary material for: Domain Agnostic Few-Shot Learning For Document Intelligence
Source: arXiv:2111.00007 source file (2021-10-29)
Supplement: Supplementary file 1 [file appendix.tex]

\section{Appendix}

\subsection{Computing Resources comparison for Tobacco-3482 data set}
As shown in Table \ref{effgnn_results_resources_tobacco} on the Tobacco-3482 dataset our model achieves a mean accuracy of 77.5 \% in par with existing baselines by utilising 470MB of DRAM capacity of the GPU with computational time of 2.5 Minutes. As shown the Table \ref{effgnn_results_resources_tobacco} our model uses merely 5 \% of memory when compared to other existing baselines such as VGG-16 which requires 8.85GB of GPU memory during training with batch size of 32 and BERT, DocBERT requiring 7.7GB and 10.5GB memory during training for batch size of 16. Our proposed framework is also efficient with regards to total computational time compared to  image based models such as VGG-16 which requires computational time of 2.30 hrs and language models such as BERT, DocBERT which requires overall computational time of approximately 6.2 hours.
\subsection{Cost comparisons for model training}
As shown in Table \ref{gnn_results_train_cost}, our framework achieved classification performance close to SOTA just by overall computational cost of 0.0058\$ using AWS T2-Micro machine and 0.05\$ using AWS T2-Micro machine for training. THis makes our framework scalable to enterprise level larger datasets. Our method can achieve same classification performance for training around 5000 images on GPU-Instance (Tesla K80 GPU) by using small computational cost of 0.4\$. As shown in Table \ref{effgnn_results_resources_tobacco} our GPU utilization is quite small when compared to other methods which gives leverage of increasing the batch size during training and inference for larger datasets or same instance can be utilized for multiple tasks based on type of model deployment during production. Other SOTA methods such as VGG-16 requires computational cost of 2.25\$ which is nearly 6 times as much as our framework on GPU and BERT,DocBERT requires computational cost of 5.4\$, 5.6\$ which is nearly 10X times compared our framework on GPU.

\begin{table}[h]
\begin{tabular}{||c |c| c ||} 
 \hline
 \textbf{Instance Type} &\textbf{ Method} & \textbf{Training Cost}
 \\ [0.5ex] 
 \hline\hline
 T2.Micro & Eff-GNN &  0.0058 \$ \\ 
 \hline
 C-Type & Eff-GNN & 0.05 \$  \\
 \hline
 Tesla K80 GPU & Eff-GNN & 0.4 \$  \\
 \hline
  Tesla K80 GPU & BERT & 5.4 \$  \\
 \hline
 Tesla K80 GPU & DOCBERT & 5.6 \$ \\ 
 \hline
 Tesla K80 GPU & VGG-16 & 2.25 \$  \\ [1ex] 
 \hline
\end{tabular}
\caption{\textbf{Table. Cost Comparison of model training and inference (5,000 images)} Note: %All costs are w.r.t Instance types not w.r.t to utilization
}
\label{gnn_results_train_cost}

%https://stackoverflow.com/questions/1673942/latex-table-positioning

\end{table}

\begin{table*}[h]
\begin{tabular}{cccccc}
\toprule
       \textbf{Tobacco (3842)} & \textbf{Batch Size} & \textbf{Epochs} & \textbf{ Train Time} & \textbf{GPU Memory(Training)} & \textbf{Inference Time}  \\
\midrule
 VGG & 32 & 38 & 1.5 hours &  8.85GB  &  21 seconds \\
 Eff-GNN (GPU) &  32 & 50 &  2.5 mins.  & \shortstack[l]{\newline \\ \newline \\ 470MB + 3.5 GB } & 0.578 seconds \\
 Eff-GNN (CPU) &  32 & 50 &  3.9 mins. & NA & 0.578 seconds \\
 DocBert & 16 & 30 & 2.3 hours &  10.5GB  & NaN \\
 BERT & 16 & 30 & 2.2 hours & 7.7GB & 7.2 seconds  \\
\bottomrule
\end{tabular}
\caption{\textbf{Memory, hardware and time required by different models on the Tobacco-3482 dataset. The numbers are reported on training 2482 images and inference for 800 Images.}}
\label{effgnn_results_resources_tobacco}
\end{table*}

%\clearpage
